# Supplementary material for: Parameterized Algebraic Protocols
Source: arXiv:2304.03764 source file (2023-04-07)
Supplement: Supplementary file 1 [file old-appendix.tex]

\appendix

\section{Extra Stuff}
\label{sec:extra-stuff}

Pragmatically interesting things that would water down the paper.

\subsection{Multiplicities}
\label{sec:multiplicities}

In practice, we want to distinguish between linear and unrestricted
data. It is straightforward though tedious to integrate the extra
information required into the type system.

Kinds $\kind$ determine the ways in which types can be used. 
Multiplicities $m$ describe the number of times a value can be used: exactly once
for $\lin$ and zero or more times for $\un$. Multiplicities can only
be combined with prekinds $\kinds$ and $\kindt$.

\begin{align*}
  \prekind &::= \kinds & \text{session types} \\
           & \mid \kindt & \text{value types} \\
  \kind &::= \kindp  & \text{protocol types} \\
   &\mid \prekind^m  & \text{prekind with multiplicity} \\
  m &::= \lin & \text{exactly one use} \\
  & \mid \un & \text{zero or more uses}
\end{align*}


We have subkinding generated by an ordering on prekinds and
multiplicities:
\pt{Not sure if $\kindp$ should be the top or if
  there should be an explicit conversion into $\kindp$.}


\begin{center}
  \begin{tikzpicture}[scale=.67]
    \node (PKT) at (0,1) {$\kindt$};
%     \node (PKM) at (0,0) {$\kindm$};
    \node (PKS) at (0,-1) {$\kinds$};
    \draw (PKS) -- (PKT) ;
%    \draw (PKM) -- (PKT) ;
  \end{tikzpicture}
  \qquad
  \begin{tikzpicture}[scale=.67]
    \node (LIN) at (0,1) {$\lin$};
    \node (UN) at (0,0) {$\un$};
    \draw (LIN) -- (UN) ;
  \end{tikzpicture}
  \qquad
  \begin{tikzpicture}[scale=.67]
    \node (PP) at (0,2) {$\kindp$};
    \node (TL) at (0,1) {$\kindtl$};
    \node (TU) at (0,0) {$\kindtu$};
    \node (SL) at (-2,-1) {$\kindsl$};
    \node (SU) at (-2,-2) {$\kindsu$};
    % \node (ML) at (-1,0) {$\kindml$};
    % \node (MU) at (-1,-1) {$\kindmu$};
    \draw (PP) -- (TL);
    \draw (TL) -- (TU);
    \draw (TL) -- (SL);
    % \draw (TL) -- (ML);
    % \draw (TU) -- (MU);
    % \draw (ML) -- (MU);
    \draw (TU) -- (SU);
    \draw (SL) -- (SU);
    % \draw (ML) -- (SL);
    % \draw (MU) -- (SU);
  \end{tikzpicture}
\end{center}


Algebraic protocol types $\proto$ are defined analogously to algebraic
datatypes. They may be parametric and the parameters $\typec{\overline\alpha}$ can have
arbitrary kinds. The metavariable $\constr$ ranges over constructor names
and metavariable $O$ ranges over polarized types, 
i.e., types adorned with a polarity $\pm$.
\begin{gather*}
  \protocolsfull
\end{gather*}
The thus defined type $\proto$ can always serve as a protocol, but in
certain cases it can also serve as a datatype definition. To this end,
we define a relation that assigns a kind to a protocol type. The kind
may be $\kindtu$ for an unrestricted datatype, $\kindtl$ for a
datatype with linear components, and $\kindp$ for a pure protocol that
does not correspond to an algebraic datatype. While an algebraic
datatype classifies values, a protocol type classifies behavior, only. 

For a data protocol, we can indicate our intent by using the $\datak$
keyword instead of $\protocolk$. Moreover, all parameters must be
proper types, not protocols.
\begin{gather*}
  \protocolsdata
\end{gather*}

\clearpage
\subsection{Protocol Definitions}
\label{sec:decl-spec-prot}


We start with a declarative rule set to determine well-formedness of a
protocol definition.

A kind context $\Delta$ maps type variables to kinds and protocol
names to (restricted, first order) arrow kinds.
% A program $\Pi$ is a sequence of protocol
% definitions ending in an expression:
\pt{We could have a separate environment for the $\proto$s}
\begin{align*}
  \Delta & ::=  \cdot
           \mid \Delta, \alpha\colon\kind
           \mid \Delta,  \proto\colon \overline\kind \to \kind
  % \\
  % \Pi & ::= M
  %       \mid \protocolsfull; \Pi
\end{align*}
We check a single protocol definition as follows where $\Delta$ may
refer to previously defined protocols:\footnote{For mutually
  recursive protocols $\overline\proto$, we would have to add the
  assumptions for all $\overline\proto$ when checking each individual $\proto_i$.}
\begin{mathpar}
  \inferrule{
    \protocolsfull \\
    (\forall i)~\typeSynth[\Delta, \proto\colon \overline{\kind} \to \kind, \overline{\alpha}\colon\overline{\kind}]
    {{\constr_i\ \overline{O_i}}}{
      \kind}
  }{
    \typeSynth{\proto} {\overline\kind \to \kind}
  }
\end{mathpar}
The judgment $ \typeSynth{{\constr\ \overline{O}}} \kind$ specifies a
valid constructor clause. It refers to type formation $\typeSynth T \kind$:
\begin{mathpar}
  \inferrule{
    \typeSynth {\overline O}  {\kind}
  }{
    \typeSynth{{\constr\ \overline{O}}} \kind
  }
\end{mathpar}

The corresponding algorithmic judgments compute the least kind for a protocol.
\begin{mathpar}
  \inferrule{
    \typeSynth {\overline O}  {\overline\kind}
  }{
    \typeSynth{{\constr\ \overline{O}}} {\klub\{\kindtu, \overline\kind\}}
  }

  \inferrule{
    \protocolsfull \\\\
    (\forall i)~\typeSynth[\Delta, \proto\colon \overline{\kind} \to \kindtu, \overline{\alpha}\colon\overline{\kind}]
    {{\constr_i\ \overline{O_i}}}{
      \kind_i} \\
    \kind = \klub_i\{\kindtu, \kind_i\}    
  }{
    \typeSynth{\proto} {\overline\kind \to \kind}
  }
\end{mathpar}
Technically, we should compute the kind $\kind$  by fixed point
iteration. For the simply recursive case, one iteration starting from
$\bot = \kindtu$ is sufficient. For mutually recursive protocols, we
have to perform a fixed point iteration as the kind of one (entry
point to a) protocol
may influence the kind of another.

\begin{example}
\begin{lstlisting}
protocol List a:TU = Nil | Cons a (List a)
\end{lstlisting}
  We have the following algorithmic derivation. Let $\Delta =
  \types{List} : \kindtu \to \kindtu, \types{a} : \kindtu$.
  \begin{mathpar}
    \inferrule*{
      \typeSynth{ \exps{Nil} }{ \kindtu} \\
      \inferrule*{\typeSynth{\types{a}}{\kindtu} \\
      \typeSynth{\types{List a}}{\kindtu}}
      {\typeSynth{ \exps{Cons}\ \types{a}\ \types{(List a)}}{\kindtu}}
    }{
      \typeSynth[]{ \types{List} }{\kindtu \to \kindtu}
    }
  \end{mathpar}

\begin{lstlisting}
protocol Neg = Neg +Int -Int
\end{lstlisting}
  We set $ \Delta = \types{Neg} : () \to \kindtu$ and obtain the derivation:
  \begin{mathpar}
    \inferrule*{
      \inferrule*{
        \inferrule*{\typeSynth{\types{Int}}{\kindtu}}{\typeSynth{\types{+Int}}{\kindtu}} \\
        \inferrule*{\typeSynth{\types{Int}}{\kindtu}}{\typeSynth{\types{-Int}}{\kindp}}
      }{
        \typeSynth{\exps{Neg}\ \types{+Int}\ \types{-Int}}{\kindp}}
    }{
      \typeSynth[]{\types{Neg}}{() \to \kindp}
    }
  \end{mathpar}
\end{example}


\subsection{Obsolete}
\label{sec:obsolete}


Define a least upper bound operation on kinds according to the Hasse diagram (incomplete):
\begin{align*}
  \kindp \klub \kind & = \kind \klub \kindp = \kindp
  & \dots
\end{align*}
\begin{gather*}
  \spec (\kindc{\overline \kind}) = \klub\{\overline\kind\}
  % \begin{cases}
  %   \kindp & \text{if any } \kindc{\kind_i} = \kindp \\
  %   \kindc{\kindt^m} & \text{if all } \kindc{\kind_i} = \kindc{\kindt^m}
  % \end{cases}
\end{gather*}

A valid constructor clause is specified by the relation $ \Delta \vdash \typec{{\constr\
    \overline{O}}} \triangleright \kind$ which refers to type formation
$\typeSynth T \kind$:
\begin{mathpar}
  % \inferrule{
  %   \typeSynth T \kind
  % }{
  %   \Delta \vdash \pneg T \triangleright \kindp
  % }
  %   
  % \inferrule{
  %   \typeSynth T \kind
  % }{
  %   \Delta \vdash \ppos T \triangleright \kind
  % }
  %   
  % \inferrule{
  %   \Delta \vdash T : \kindg
  % }{
  %   \Delta \vdash T^\circ \triangleright \kindp
  % }
  %   
  % \inferrule{
  %    \typeSynth T  \kindp
  % }{
  %   \Delta \vdash \ppos T \triangleright \kindp
  % }
  %   
  \inferrule{
    \typeSynth {\overline O}  {\overline\kind}
  }{
    \Delta \vdash \typec{{\constr\ \overline{O}}} \triangleright \klub\{\overline\kind\}
  }
\end{mathpar}
%

The kind of a protocol definition is calculated as a fixed point. For
recursive uses of the protocol $\proto$ we assume a certain kind $\kind$
when calculating the kind $\kind_i$ resulting from each
constructor. The assumed kind $\kind$ must be the least upper bound of
the constructor kinds.
\begin{mathpar}
  \inferrule{
    % \protocolsfull \triangleright \kind \\
    (\forall i)~[\vdash\typec{\proto\ \overline{\alpha}\colon \kind}]~\overline{\alpha}\colon\overline{\kind} \vdash
    \typec{{\constr_i\ \overline{O_i}}} \triangleright
    \kind_i \\
    \kind = \klub\{\kind_i\}
  }{
    \protocolsfull \triangleright \kind
  }
  % 
  % \inferrule{
  %   \overline{\alpha\colon\kindg},
  %   \overline{\beta\colon\kindt} \vdash \typec{T_i} : \kindg
  %   \quad\text{or}\quad
  %   \overline{\alpha\colon\kindg},
  %   \overline{\beta\colon\kindt} \vdash \typec{T_i}^\pm : \kindt
  % }{ \protocolsfull \triangleright \kind}
\end{mathpar}
%
\vv{Something fishy here: the protocol term in the conclusion is exactly that of
  the premise. Also, it is not obvious what the $C$ and the $O$ in the 2nd
  premise refer to. If they should be added to the conclusion, then need we not
  a base rule (a rule for an empty---or singleton---protocol)? Finally, perhaps
  the 2nd and 3rd premise and the 5th $\triangleright$-rule can be combined into
  one premise only.}
\pt{Added two sentences of explanation and slightly rephrased the formula.}

For algorithmic checking, we assume the  least restrictive
kind $\kindtu$ for $\proto\ \overline\alpha$ and then recalculate with the kind that is calculated by $\spec
(\overline\kind)$ in the rule until we reach a fixpoint. This 
approach terminates as it amounts to calculating a fixed point in the finite
lattice of kinds. For $n$ mutually recursive definitions, we start with the same
minimal assumptions, but may have to iterate $n$ times to reach the fixed point.
%
\vv{Do we simply mean that all $C_i\overline{O_i}$ must have the same
  $\spec(\overline\kind)$? Something like this\dots
\begin{mathpar}
  \inferrule{
    % \overline{\typec\alpha}\colon\overline{\kindg},
    % \overline{\typec\beta}\colon\overline{\kindc{\kindt^m}} 
    \Delta
    \vdash
    \typec{\termc{\constr_i}\ \overline O_i} \triangleright
    \spec(\overline\kind)
  }{
\protocolk\ \typec{\proto\ (
    % \typec{\overline{\alpha}\colon \overline\kindg,
    % \overline{\beta}\colon\overline{\kindc{\kindt^m}}
  \Delta
    )}~\blk{=}~\typec{\termc{\constr_1}\
    \overline O_1\mid\dots\mid\termc{\constr_n}\ \overline O_n}
 \triangleright \kind
}
\end{mathpar}
} % \vv
\pt{No. Constructors can indicate different kinds. For example, a
  unidirectional constructor like \texttt{Nil} pushes the kind to
  $\kindtl$ and a constructor with a negative argument  pushes the
  kind to $\kindp$.}
\am{Wouldn't this be equivalent to what Vasco is proposing, considering
    the subkinding relation (and assuming that $\kindp$ is in the top of the 
    hierarchy)? Being equivalent, I don't have any preference.}


Intuitively, if there are any parameters
annotated with $\pneg{}$, then we
have $\typec{\proto\ \overline{T}} : \kindp$, i.e., $\kind = \kindp$.
Otherwise we have $\kind = \kindt^m$, as such a protocol also makes
sense as pure data. Here is the corresponding specialized rule for
pure datatypes:
\begin{mathpar}
  \inferrule{
    \overline{\typec\alpha}\colon\overline{\kindc{\kindt^m}} \vdash \typec{O_i} : \kindc{\kindt^m}
  }{ \protocolsdata \triangleright \kindc{\kindt^m} }
\end{mathpar}
\vv{This rule makes sense. Should the premise read $\overline{\ppos{T_i}}$?}
\pt{No, definitely not. The premise is plain type formation.}
\pt{This is up for discussion: We assume that we cannot communicate
  functions and channels as primitive types.}



\subsection{Functions in Messages}
\label{sec:functions-messages}

We can classify a function's type as a message type, if all free
variable of the function are message types. To express this feature,
we have to extend the arrow type to carry an annotation of the form
$\prekind^m$ as in the following formation rules:
\begin{mathpar}
    \infrule{\textcolor{red}{\rulenametypeArrow}}{
    \typeSynth T \kindtl
    \\ \typeSynth U \kindtl
    \\ \kindmu \le \kind
    \\ \kind = \prekind^\mult
  }{
    \typeSynth{\TFun[\kind] T U}{\kind}}
    
  \infrule{\textcolor{red}{\rulenametypePoly}}{
    \typeSynth[\Delta,\typec{\alpha}\colon\kind']{\typec{T}}{\kind}
    \\ \kindmu \le \kind
    % \\ \kind = \kindt^m 
  }{
    \typeSynth{\forall (\typec{\alpha}\colon\kind') \typec{T}}{\kind}}
\end{mathpar}
This rule for polymorphism enables the transmission of polymorphic
functions.

The expression typing for lambda expressions needs to be adapted:
\begin{mathpar}
    \infrule{\textcolor{red}{\rulenameexpAbs-Msg}}
  {\typeSynth{T}{\_} \\ \expSynth{\Gamma_1,
      x\colon\typec{T}}{e}{U}{\Gamma_2} \\
    \termc y \in \FVE{\termc e}, \termc y\ne \termc x \Rightarrow \typeSynth{\Gamma_1 (\termc y)}{\kindml}
  }
  {\expSynth{\Gamma_1}{\abse[\kindml]xTe}{\TFun[\kindml]{T}{U}}{\Gamma_2 \div \termc{x}}}
\end{mathpar}

\subsection{Type Isomorphism}
\label{sec:type-isomorphism}


Consider universally quantified types modules type isomorphism (see
Roberto Di Cosmo's work).
This amounts to adding this conversion rule to the declarative type system:
\begin{mathpar}
  \infrule{\textcolor{red}{\rulenametconvAll}}{
    \typec\alpha\notin \FVT{\typec T}
  }{
    \isConv{\TForall\alpha\kind{\TFun T U}}{{\TFun T
        {\TForall\alpha\kind U}}} \kindt
  }
\end{mathpar}
The algorithmic system can be adapted easily:
\begin{mathpar}
    \infrule{\textcolor{red}{\rulenameexpAppAll}}
  {\expSynth{\Gamma_1}{e_1}{\TForall{\overline\alpha}{\overline\kind}{\TFun{T_1}{T_2}}}{\Gamma_2}
    \\\typec{\overline\alpha}\notin \FVT{\typec{T_1}}
    \\\expAgainst{\Gamma_2}{e_2}{T_1}{\Gamma_3}} 
  {\expSynth{\Gamma_1}{\appe {e_1}{e_2}}{\TForall{\overline\alpha}{\overline\kind} {T_2}}{\Gamma_3}}

  \infrule{\textcolor{red}{\rulenameexpTApp}}
  {\expSynth{\Gamma_1}{e}{\TFun[\overline{m}]{\overline U}{\TForall \alpha\kind U}}{\Gamma_2} \\ \typeAgainst{T}{\kind}} 
  {\expSynth{\Gamma_1}{\tappe e T}{\TFun[\overline{m}]{\overline U} {(U\tsubs{T}{\alpha})}}{\Gamma_2}}
\end{mathpar}
Normal-form calculation has to be adjusted accordingly. The one rule concerned
with \(\TForall{\alpha}{\kind}{T}\) is replaced by
\begin{mathpar}
  \inferrule{
    \text{\textit{pushable}}(\typec{\overline\alpha}, \TFun TU) \\
    \Normal[+] T = \typec{T'} \\
    \Normal[+]{\TForall{\overline\alpha}{\overline\kind}U} = \typec{U'}
  }{
    \Normal[+]{\TForall{\overline\alpha}{\overline\kind}{\TFun TU}} =
      \TFun{T'}{U'}
  }

  \inferrule{
    \neg \text{\textit{pushable}}(\typec\alpha, \typec T) \\
    \Normal T = \typec{T'}
  }{
    \Normal{\TForall \alpha \kind T} =
      \TForall{\alpha}{\kind}{\typec{T'}}
  }
\end{mathpar}
where
\[
  \text{\textit{pushable}}(\typec{\overline{\alpha}}, \typec{T}) \coloneqq
    \begin{array}{ll}
      \typec{T}=\TFun UV \wedge \typec{\overline\alpha} \not\in \FVT{\typec U}
        & \text{for any}~\typec U,\typec V \\
    \end{array}
\]

%%% Local Variables:
%%% mode: latex
%%% TeX-master: "main"
%%% End:
